# Supplementary material for: Beating the random assignment on constraint satisfaction problems of bounded degree
Source: arXiv:1505.03424 source file (2015-08-11)
Supplement: Supplementary file 1 [file appendix.tex]

%%% Local Variables:
%%% mode: latex
%%% TeX-master: "../lowdegcsp"
%%% End:
